# Supplementary material for: Improved Lower Bound on DHP: Towards the Equivalence of DHP and DLP for Important Elliptic Curves Used for Implementation
Source: arXiv:1610.01354 source file (2016-11-26)
Supplement: Supplementary file 1 [file Arxiv_appendices.tex]

\documentclass[a4paper,10pt]{article}
\usepackage[utf8]{inputenc}
\usepackage{amssymb, amsthm}
\usepackage{amsmath}
\usepackage{graphicx}
\graphicspath{ {Images/} }
 \textwidth 4.75 in  \textheight 8.25 in
\usepackage{cite}

\usepackage[toc,page]{appendix}
%opening
\title{Appendices for \textquotedblleft Improved Lower Bound on DHP: 
Towards the Equivalence of DHP and DLP for Important Elliptic Curves Used for Implementation \textquotedblright}
\author{Prabhat Kushwaha}

\begin{document}
\bibliographystyle{plain}

\maketitle

\begin{appendices}

\section{Elliptic curve domain parameters over prime field}

The following data present several SECG curves\cite{secg} which are defined over some prime field of characteristic not equal 
to $2$ and are used for practical purposes. For these curves, prime $p$ denotes the order of the elliptic curve group 
and $d$ is the suitable divisor of $p-1$ which is used by us for various computation in Table 1. 	

\subsection{SECP112R1}
$p = 4451685225093714776491891542548933$ \newline
$d = 140876$

\subsection{SECP112R2}
$p = 1112921306273428674967732714786891$ \newline
$d = 110852811870$

\subsection{SECP128R1}
$p = 340282366762482138443322565580356624661$
\newline
$d = 9476076960994$

\subsection{SECP128R2}
$p = 85070591690620534603955721926813660579$
\newline
$d = 3101689558$

\subsection{SECP160K1}
$p = 1461501637330902918203686915170869725397159163571$
\newline
$d = 42918291593381467397$

\subsection{SECP160R1}
$p = 1461501637330902918203687197606826779884643492439$
\newline
$d = 22167198845997443 $

\subsection{SECP160R2}
$p = 1461501637330902918203685083571792140653176136043$
\newline
$d = 142004808588765074419$

\subsection{SECP192K1}
$p = 6277101735386680763835789423061264271957123915200845512077$
\newline
$d= 43818996$

\subsection{SECP192R1}
$p = 6277101735386680763835789423176059013767194773182842284081$
\newline
$d = 9564682313913860059195669 $

\subsection{SECP224K1}
$p = 2695994666715063979466701508701964034651032708312007454899$ \newline
$4958668279$
\newline
Appropriate size of divisor $d$ of $p-1$ not available

\subsection{SECP224R1}
$p = 2695994666715063979466701508701962594045780771442439172168$ \newline 
$2722368061$
\newline
$d = 533642580$

\subsection{SECP256K1}
$p=1157920892373161954235709850086879078528375642790749043826$ \newline
$05163141518161494337$ \newline
$d = 65709355417112419152054124 $

\subsection{SECP256R1}
$p = 115792089210356248762697446949407573529996955224135760$ \newline
$342422259061068512044369$ \newline
$d = 71482998987075857096374359 $

\subsection{SECP384R1}
$p = 3940200619639447921227904010014361380507973927046544666 794$ \newline
$6905279627659399113263569398956308152294913554433653942643$ \newline
$d = 12895580879789762060783039592702$

\subsection{SECP521R1}
$p = 686479766013060971498190079908139321726943530014330540939 4463 $ \newline
$45918554318339765539424505774633321719753296399637136332111 386476$ \newline
$ 8612440380340372808892707005449$ \newline
$d = 1898873518475180724503002533770555108536 $

\section{ Elliptic curve domain parameters over $\mathbb{F}_{2^m}$}
The following data present several SECG curves\cite{secg} which are defined over a binary field and are used for practical
purposes. For these curves, prime $p$ is the largest divisor of the order of that particular elliptic curve group(with a very small
co-factor of either 2 or 4) and $d$ is the appropriate divisor of $p-1$  used by us for various computation in Table 2.

\subsection{SECT113R1}
$p = 5192296858534827689835882578830703 $ \newline
$d =253877289037 $

\subsection{SECT113R2}
$p = 5192296858534827702972497909952403 $ \newline
$d = 215851796187 $
\subsection{SECT131R1}
$p= 1361129467683753853893932755685365560653 $\newline
$d = 23348 $

\subsection{SECT131R2}
$p = 1361129467683753853879535043412812867983 $ \newline
$d = 485524729 $

\subsection{SECT163K1}
$p = 5846006549323611672814741753598448348329118574063 $ \newline
$d = 33118034411893094 $ 

\subsection{SECT163R1}
$p = 5846006549323611672814738465098798981304420411291 $ \newline
$d = 27744064547201903 $

\subsection{SECT163R2}
$p = 5846006549323611672814742442876390689256843201587 $ \newline
$d = 859825042 $

\subsection{SECT193R1}
$p = 6277101735386680763835789423269548053691575186051040197193 $ \newline
$d = 1697589986603916123127 $

\subsection{SECT193R2}
$p = 6277101735386680763835789423314955362437298222279840143829 $ \newline
$d = 4345632155805272808276901 $

\subsection{SECT233K1}
$p = 34508731733952818937173779311385127605709409888622521263280$ \newline 
$87024741343 $ \newline
$d = 11064269030135607689238 $

\subsection{SECT233R1}
$p = 6901746346790563787434755862277025555839812737345013555379$ \newline
$383634485463 $ \newline
$d = 443484653691663066996649 $

\subsection{SECT239K1}
$p = 22085588309729804119791218759286481494821656132170984888$ \newline
$7480219215362213 $ \newline
$d = 912013207122974008798076 $

\subsection{SECT283K1}
$p = 38853377844514581418389238136470378132848117337930613242$ \newline 
$95874997529815829704422603873 $ \newline
$d = 19578145037471479248182334822 $

\subsection{SECT283R1}
$p = 7770675568902916283677847627294075626569625924376904889$ \newline
$109196526770044277787378692871 $ \newline
$d = 34107744933314238426752172695 $

\subsection{SECT409K1}
$p = 3305279843951242994759576540163855199142023414821406096$ \newline
$42324395022880711289249191050673258457777458014096366590617$ \newline
$731358671 $ \newline
$d = 572443222870261113609193333057890 $

\subsection{SECT409R1}
$p = 6610559687902485989519153080327710398284046829642812192$ \newline 
$84648798304157774827374805208143723762179110965979867288366$ \newline
$567526771 $ \newline
$d = 133035142307481057108300314154446543724338 $

\subsection{SECT571K1}
$p = 19322 68761 50862 91723 47675 94546 59936 72149 46366 48532 17499$ \newline
$ 32861 76257 25759 57114 47802 12268 13397 85227 06711 83470 67128 0082$ \newline
$5 35146 12736 74974 06661 73119 29682 42161 70925 03555 73368 52766 73$ \newline
$d = 16508 36032 27521 05262 55468 05906 33369 14554 24949 78266 76631 916 $

\subsection{SECT571R1}
$p = 38645 37523 01725 83446 95351 89093 19873 44298 92732 97064 34998 65$ \newline
$723 52514 51519 14228 95604 24536 14399 93894 15773 08313 38811  21926 944$ \newline
$48 62468 72462 81681 30702 34528 28830 33324 11393 19110 52857 03$ \newline
$d = 21606 77396 58822 05526 51437 94633 89966 05699 04327 74077 55096 919 $
\end{appendices}
\bibliography{Arxiv_appendices}
\end{document}
